# Supplementary material for: Tuning Hydrogen Adsorption and Electronic Properties from Graphene to Fluorographone
Source: arXiv:2005.03854 source file (2020-05-08)
Supplement: Supplementary file 1 [file Schleder_SupportingInformation.pdf]

## Supporting Information

# Tuning Hydrogen Adsorption and Electronic Properties from Graphene to Fluorographone


Gabriel R. Schleder [1,*] Enesio Marinho Jr [1,†] Douglas J. R. Baquiao [1] Yuri M. Celaschi [1] Felipe Gollino [2] Gustavo M. Dalpian [1] and Pedro A. S. Autreto [1,‡]

[1] *Federal University of ABC (UFABC), 09210-580 Santo André, São Paulo, Brazil*

[2] *São Carlos Institute of Chemistry, University of São Paulo, 13566-590 São Carlos, São Paulo, Brazil*

* gabriel.schleder@ufabc.edu.br

† enesio.junior@ufabc.edu.br

‡ pedro.autreto@ufabc.edu.br

## I. REACTIVE MOLECULAR DYNAMICS STRUCTURES

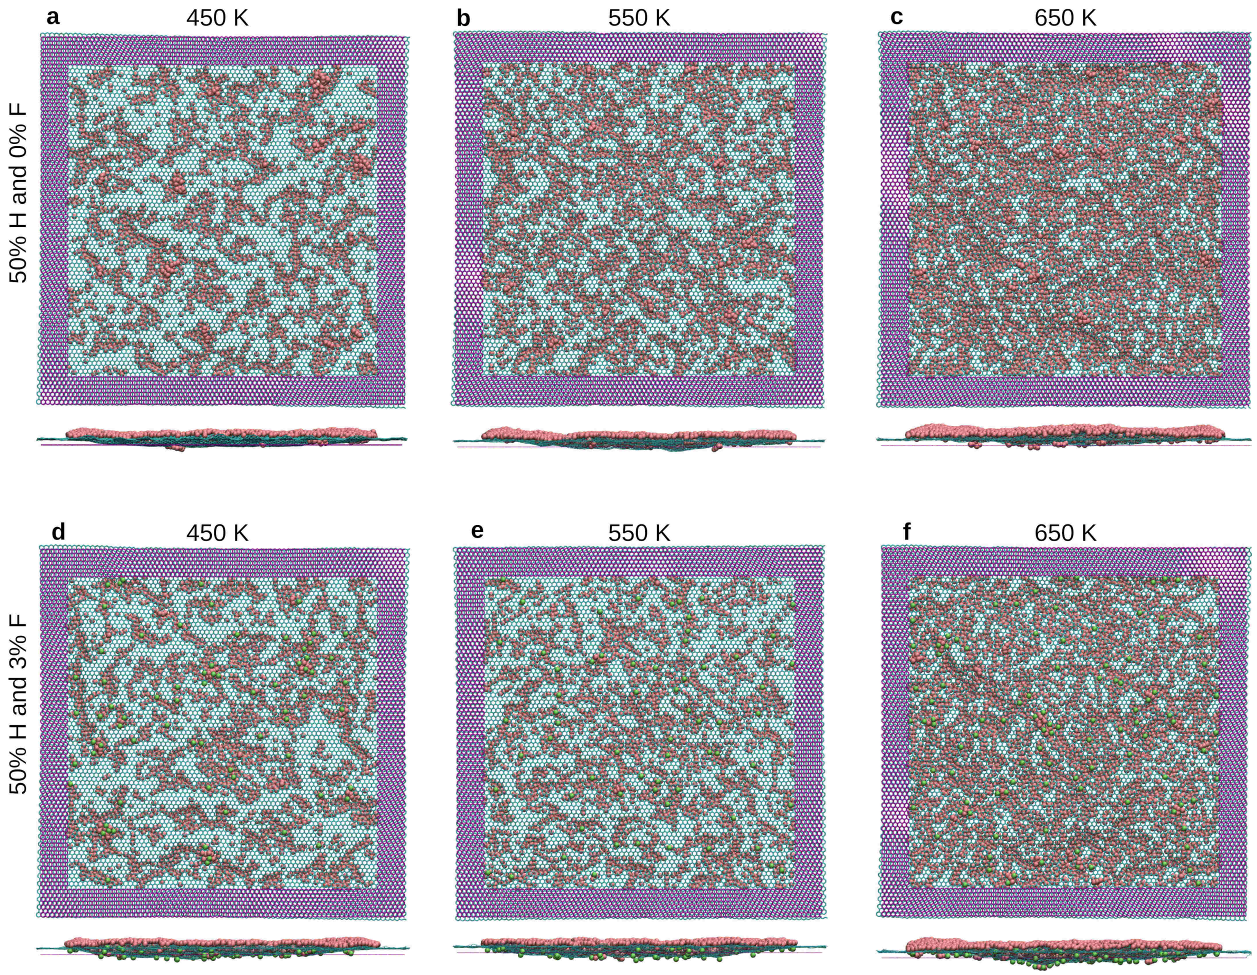


FIG. 1. Final configurations obtained from reactive molecular dynamics simulations: (a) 0% F at 450 K, (b) 0% F at 550 K, (c) 0% F at 650 K, (d) 3% F at 450 K, (e) 3% F at 550 K, (f) 3% F at 650 K. The graphene sheet used, and presented in the manuscript Figure 1, is composed of 15744 carbon atoms. The initial atmosphere used is composed of 50% hydrogen (corresponding to 7872 atoms), in conditions with or without 7.5% fluorine (corresponding to 1180 atoms). The adsorbed percentage during the molecular dynamics is presented in manuscript Figure 6.

## II. PAIR DISTRIBUTION FUNCTION (PDF)

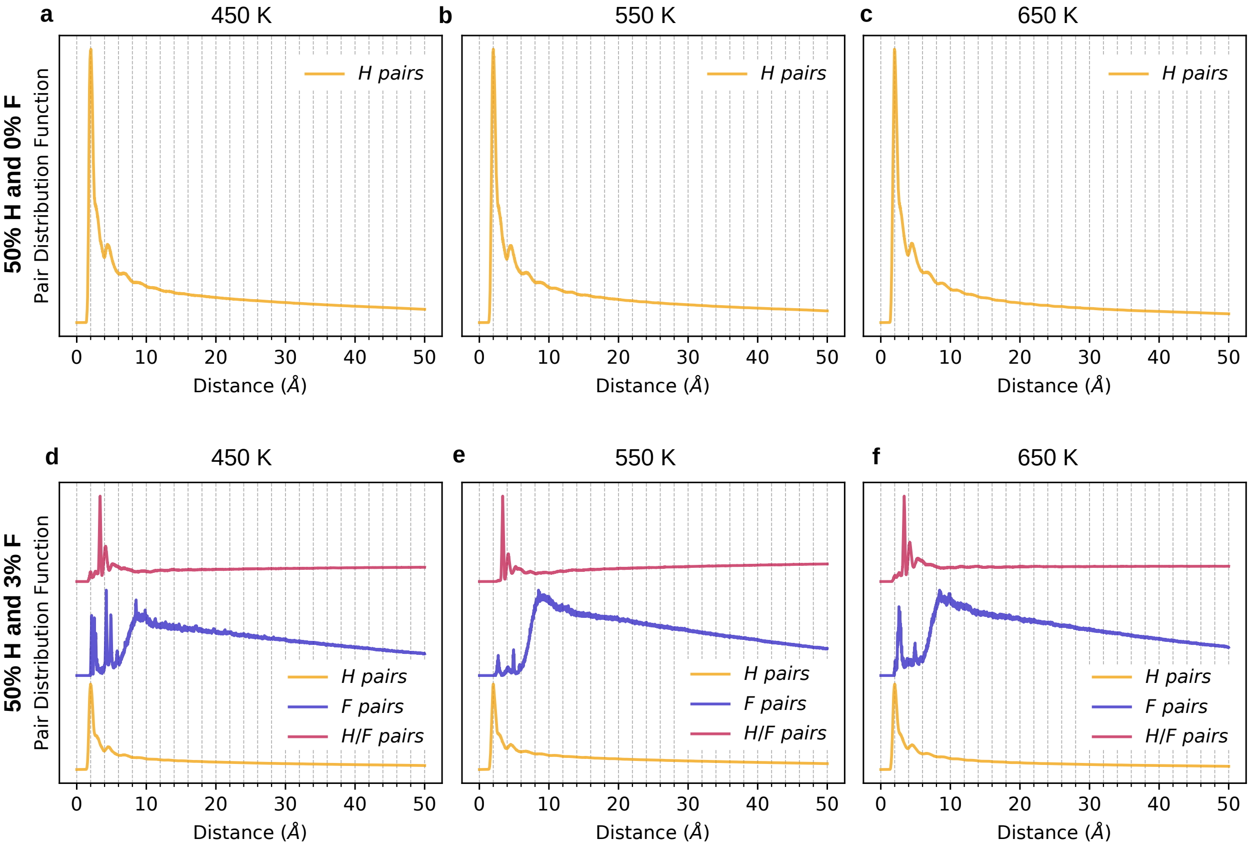


FIG. 2. Pair distribution functions (PDF) of the final configurations obtained from reactive molecular dynamics simulations: (a) 0% F at 450 K, (b) 0% F at 550 K, (c) 0% F at 650 K, (d) 3% F at 450 K, (e) 3% F at 550 K, (f) 3% F at 650 K. Yellow, blue, and red colors indicate the correlations between H/H, F/F, and H/F pairs, respectively. The PDF $g(r)$ were calculated with the histogram method implemented [1] in the VMD software [2].


[1] B. G. Levine, J. E. Stone, and A. Kohlmeyer, Fast analysis of molecular dynamics trajectories with graphics processing units – Radial distribution function histogramming, Journal of Computational Physics **230**, 3556 (2011).

[2] W. Humphrey, A. Dalke, and K. Schulten, VMD: Visual molecular dynamics, Journal of Molecular Graphics **14**, 33 (1996).
